# Supplementary material for: On Termination of Polynomial Programs with Equality Conditions
Source: arXiv:1510.05201 source file (2020-09-01)
Supplement: Supplementary file 1 [file appendix.tex]

\appendix
\section{Appendix for proofs}\label{sec:appendix}
